# Supplementary material for: Spatial Name System
Source: arXiv:2210.05036 source file (2022-11-30)
Supplement: Supplementary file 1 [file 7_appendices.tex]

\begin{appendices}

\chapter{Appendix}
\label{ch-appendix}

\end{appendices}
